# Supplementary material for: LatentCRF: Continuous CRF for Efficient Latent Diffusion
Source: arXiv:2412.18596 source file (2024-12-24)
Supplement: Supplementary file 1 [file foe_filters.tex]

\begin{figure*}[t]
    \begin{minipage}{\linewidth}
        \centering\centering
        \includegraphics[width=0.95\linewidth]{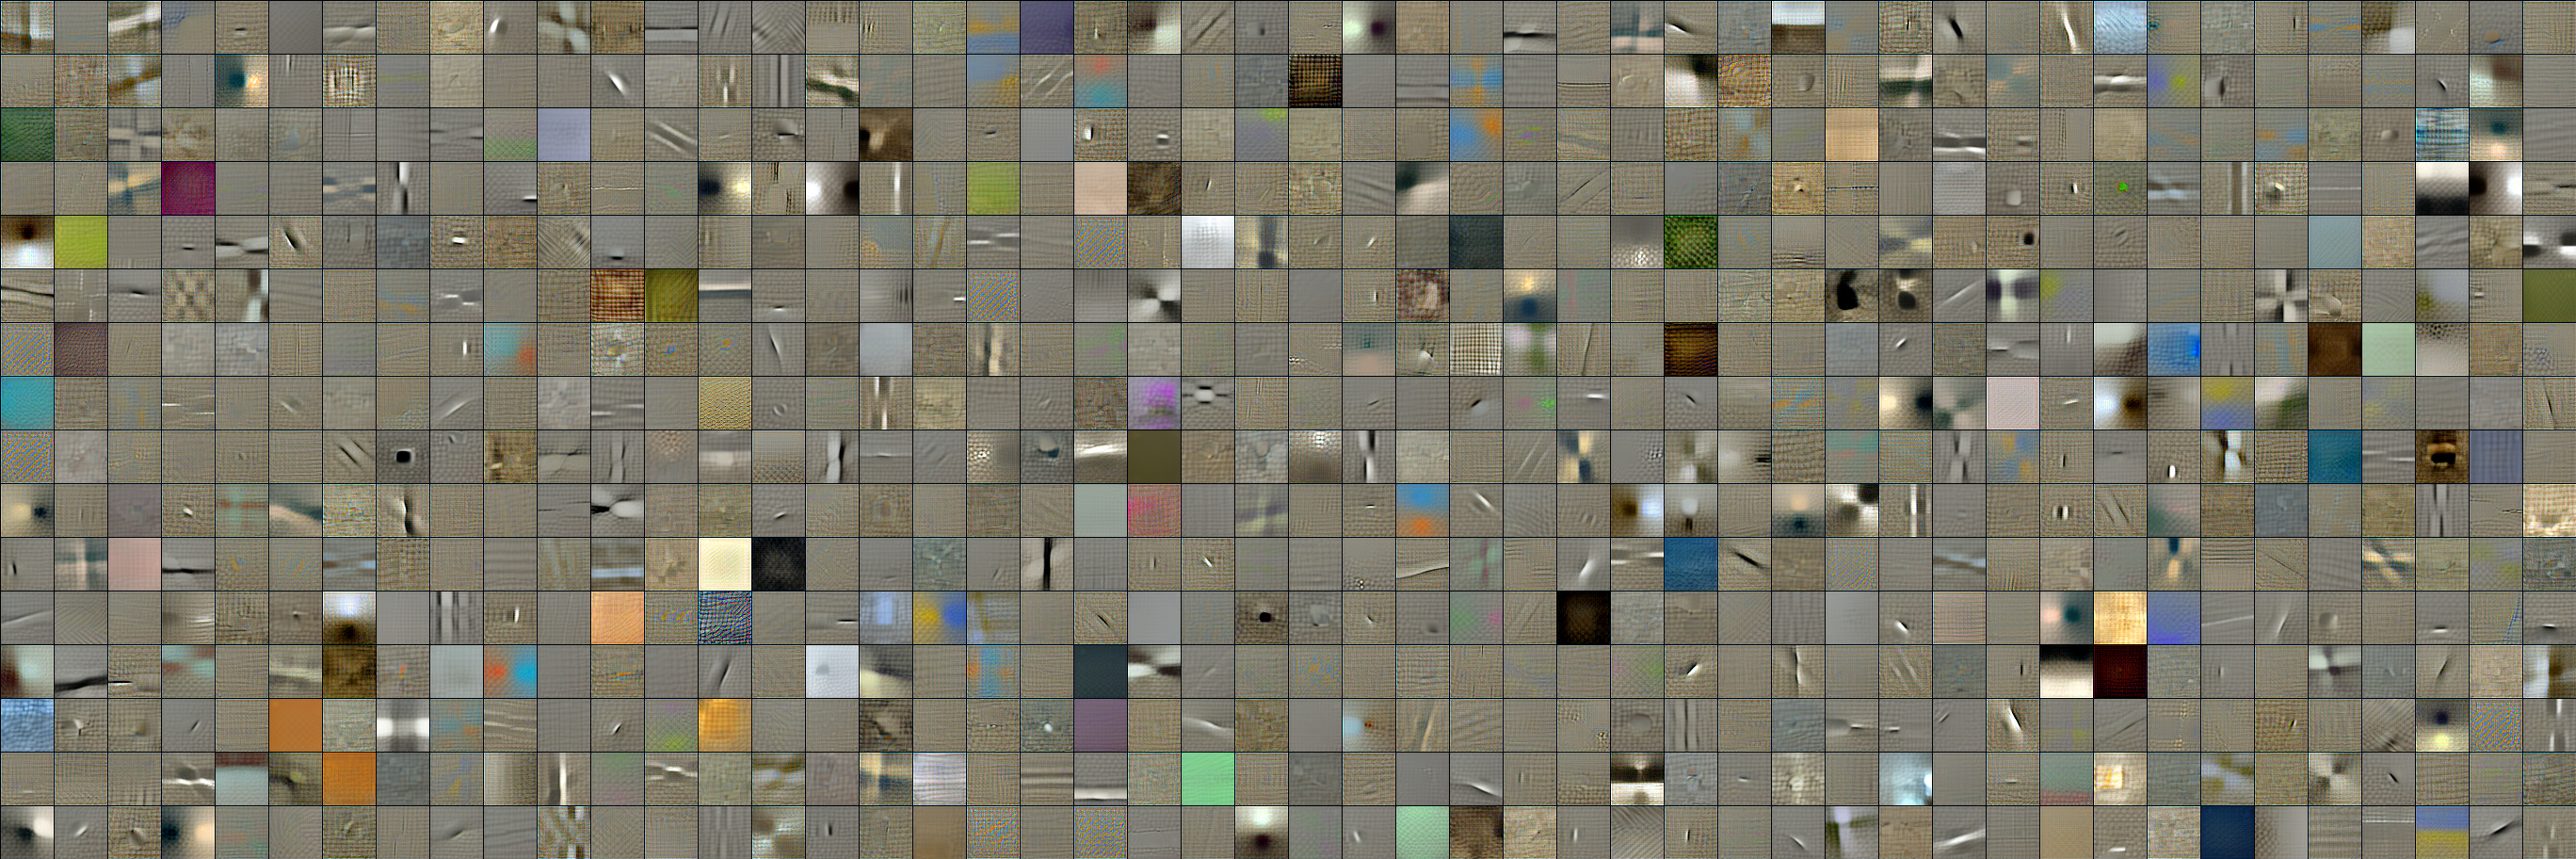}
    \end{minipage}
    \vspace{-0.5em}
    \caption{
    \textbf{Learned FoE filters:}
    \kr{describe more.}
    }
    \label{fig:app_foe_filters}
\end{figure*}
